# Supplementary material for: m4: A Learned Flow-level Network Simulator
Source: arXiv:2503.01770 source file (2025-03-03)
Supplement: Supplementary file 1 [file 8_appendix.tex]

\appendix
\section*{Appendix}
